# Supplementary material for: Scaling up self-supervised learning for improved surgical foundation models
Source: arXiv:2501.09436 source file (2025-01-16)
Supplement: Supplementary file 1 [file 8-Supplementary.tex]

%%%%%%%%%%%%%%%%%%%%%%%%%%%%%%%%%%%%%%%%%%%%%%%%%%%%%%%%%%%%%%%%%%%%%%%%%%%%%%%%%%%%%%%%%%%%%%%%%%%%%%%%%%%%%%%%%%%%%%%%%%%%%%%%%%%%%%%%%%%%%%%%%%%%%%%%%%%%%%
%%%%%%%%%%%%%%%%%%%%%%%%%%%%%%%%%%%%%%%%%%%%%%%%%%%%%%%%%%%%%%%%%% SUP. MATERIAL %%%%%%%%%%%%%%%%%%%%%%%%%%%%%%%%%%%%%%%%%%%%%%%%%%%%%%%%%%%%%%%%%%%%%%%%%%%%%
%%%%%%%%%%%%%%%%%%%%%%%%%%%%%%%%%%%%%%%%%%%%%%%%%%%%%%%%%%%%%%%%%%%%%%%%%%%%%%%%%%%%%%%%%%%%%%%%%%%%%%%%%%%%%%%%%%%%%%%%%%%%%%%%%%%%%%%%%%%%%%%%%%%%%%%%%%%%%%
% Reset section counters
\setcounter{section}{0}

\section{Data pre-processing details}
\label{sec: Supplementary-Preprocess}

%%%%%%%%%%%%%%%%%%%%%%%%%%%%%%%%%%%%%%%%%%%%%%%%%%%%%%%%%%%%%%%%%% SUBSECTION: Normalization %%%%%%%%%%%%%%%%%%%%%%%%%%%%%%%%%%%%%%%%%%%%%%%%%%%%
\subsection{Normalization}
\label{sec: Supplementary-Preprocess-Normalization}
For data concerning Barrett's neoplasia detection, the RGB channels of WLE images are normalized by the channel-wise mean $(0.64, 0.361, 0.313)$ and standard deviation $(0.189, 0.156, 0.141)$.

%%%%%%%%%%%%%%%%%%%%%%%%%%%%%%%%%%%%%%%%%%%%%%%%%%%%%%%%%%%%%%%%%% SUBSECTION: Data augmentation %%%%%%%%%%%%%%%%%%%%%%%%%%%%%%%%%%%%%%%%%%%%%%%%%%%%
\subsection{Data augmentation}
\label{sec: Supplementary-Preprocess-Augmentation}

\subsubsection{Downstream training: default N-DSA set}
The default set of data augmentation techniques applied during training and validation procedures consists of:
\begin{enumerate}[noitemsep]
\item \textit{Flip:} Flip the image horizontally and/or vertically ($p$=0.5).
\item \textit{Rotate:} Rotate the image by $\theta \in \{90^{\circ}, 180^{\circ}, 270^{\circ}\}$ ($p$=0.6). 
\item \textit{Affine:} Apply rotation of $\theta \in (-25^{\circ}, +25^{\circ})$, maximum translation of 5 times the image height and width, and shearing of $\theta \in (-15^{\circ}, +15^{\circ})$ ($p$=0.2).
\item \textit{Sharpness:} Increase sharpness with factor of 2 ($p$=0.2). 
\item \textit{Grayscale:} Convert to grayscale ($p$=0.2).
\item \textit{Gaussian blur:} Gaussian blurring with a blurring radius between 0.1 and 2 ($p$=0.2).
\item \textit{Color jitter:} Randomly adjust brightness, contrast and saturation. Factors for these aspects are sampled uniformly from either range of $[0.5, 1.5]$, $[0.7, 1.3]$ and $[0.9, 1.1]$, which is chosen randomly ($p$=0.6).
\item \textit{Random crop:} Randomly take a crop within a [0.7, 1.1] scale of the image. Patch is downscaled to the desired image size with bi-cubic interpolation ($p$=0.33).
\item \textit{Random noise:} Addition of random Gaussian noise sampled from $\mu=0$ and $\sigma^2 \in \{0.01, 0.02, 0.03, 0.05\}$ ($p$=0.5). 
\end{enumerate}

For techniques \textit{Gaussian blur} / \textit{Sharpness} / \textit{Affine} either one can be applied simultaneously, as well as for \textit{Grayscale} / \textit{Color jitter}. For validation purposes the images are randomly augmented with \textit{Rotate}, \textit{Flip} and \textit{Color jitter} with ranges $[0.7, 1.3]$ and $[0.9, 1.1]$.

\subsubsection{Downstream training: DSA set}
The domain-specific set of data augmentation techniques applied during training and validation procedures consists of:
\begin{enumerate}[noitemsep]
\item \textit{Flip:} Flip the image horizontally and/or vertically ($p$=0.5).
\item \textit{Rotate:} Rotate the image by $\theta \in \{90^{\circ}, 180^{\circ}, 270^{\circ}\}$ ($p$=0.6). 
\item \textit{Random crop:} Randomly take a crop within a [0.7, 1,1] scale of the image. Patch is downscaled to the desired image size with bi-cubic interpolation ($p$=0.33).
\item \textit{Motion blur:} Apply motion blurring with a blurring limit randomly sampled from either range of $[9, 9]$, $[11, 11]$, $[17,17]$, $[21, 21]$ and $[25, 25]$ ($p$=0.1).
\item \textit{Zoom blur:} Apply zoom blurring with a maximum factor randomly sampled from either range of $[1.01, 1.02]$, $[1.03, 1.04]$, $[1.05, 1.06]$, $[1.07, 1.08]$ and $[1.09, 1.1]$ ($p$=0.1).
\item \textit{Lens blur:} Apply lens blurring with a blurring limit randomly sampled from either range of $[1, 1]$, $[3, 3]$, $[5, 5]$, $[7, 7]$ and $[9, 9]$ ($p$=0.1).
\item \textit{Median blur:} Apply median blurring with a maximum aperture linear size randomly sampled from either range of $[1, 1]$, $[3, 3]$, $[5, 5]$, $[7, 7]$ and $[9, 9]$ ($p$=0.1).
\item \textit{Defocus blur:} Apply defocus blurring with a blurring radius randomly sampled from either range of $[9, 9]$, $[11, 11]$, $[17,17]$, $[21, 21]$ and $[25, 25]$ ($p$=0.1).
\item \textit{Increased sharpness:} Increase the sharpness with visibility and lightness of the sharpened image randomly sampled from either range of $[0.1, 0.2]$, $[0.2, 0.3]$, $[0.3, 0.4]$, $[0.4, 0.5]$ and $[0.5, 0.6]$ ($p$=0.25).
\item \textit{Decreased sharpness:} Decrease the sharpness with visibility randomly sampled from either range of $[0.1, 0.2]$, $[0.2, 0.3]$, $[0.3, 0.4]$, $[0.4, 0.5]$ and $[0.5, 0.6]$, and the Gaussian kernel size for blurring randomly sampled from either range of $[3, 3]$, $[5, 5]$, $[7, 7]$, $[9, 9]$ and $[11, 11]$ ($p$=0.25).
\item \textit{Increased contrast:} Increase contrast with factor randomly sampled from either range of $[1.01, 1.1]$, $[1.11, 1.2]$, $[1.21, 1.25]$, $[1.26, 1.3]$ and $[1.31, 1.4]$ ($p$=0.25).
\item \textit{Decreased contrast:} Decrease contrast with factor randomly sampled from either range of $[0.95, 0.99]$, $[0.9, 0.94]$, $[0.85, 0.89]$, $[0.75, 0.84]$ and $[0.65, 0.74]$ ($p$=0.25).
\item \textit{Increased brightness:} Increase brightness with factor randomly sampled from either range of $[1.01, 1.2]$, $[1.21, 1.4]$, $[1.41, 1.6]$, $[1.61, 1.8]$ and $[1.81, 2.0]$ ($p$=0.25).
\item \textit{Decreased brightness:} Decrease brightness with factor randomly sampled from either range of $[0.9, 0.99]$, $[0.85, 0.89]$, $[0.8, 0.84]$, $[0.75, 0.79]$ and $[0.7, 0.74]$ ($p$=0.25).
\item \textit{Increased saturation:} Increase saturation with factor randomly sampled from either range of $[1.01, 1.05]$, $[1.06, 1.1]$, $[1.11, 1.15]$, $[1.16, 1.2]$ and $[1.21, 1.25]$ ($p$=0.25).
\item \textit{Decreased saturation:} Decrease saturation with factor randomly sampled from either range of $[0.9, 0.99]$, $[0.8, 0.89]$, $[0.7, 0.79]$, $[0.6, 0.69]$ and $[0.5, 0.59]$ ($p$=0.25).
\item \textit{Hue red:} Apply jitter in red color spectrum with factor randomly sampled from either range of $[0.0, 0.01]$, $[0.011, 0.013]$, $[0.014, 0.016]$, $[0.017, 0.018]$ and $[0.019, 0.02]$ ($p$=0.25).
\item \textit{Hue green:} Apply jitter in green color spectrum with factor randomly sampled from either range of $[-0.01, 0.0]$, $[-0.013, -0.011]$, $[-0.016, -0.014]$, $[-0.02, -0.017]$ and $[-0.025, -0.021]$ ($p$=0.25).
\item \textit{Random noise:} Addition of random Gaussian noise sampled from $\mu=0$ and $\sigma^2 \in \{0.01, 0.02, 0.03, 0.05\}$ ($p$=0.5).
\end{enumerate}

For each of the techniques regarding blurring, sharpness, contrast, brightness, saturation and hue, only a single transform can be applied simultaneously. For validation purposes the images are augmented with randomly sampled ranges up to the third option of each transform.

\subsubsection{Domain-specific SSL pre-training: default N-DSA set}
The default set of data augmentation techniques in the DINO SSL framework~\citep{DINO} applied during pre-training consists of:
\begin{enumerate}[noitemsep]
\item \textit{Random crop global:} Randomly take a crop within a [0.4, 1.0] scale of the image. Patch is downscaled to the desired image size (256$\times$256) with bi-cubic interpolation ($p$=1).
\item \textit{Random crop local:} Randomly take a crop within a [0.05, 0.4] scale of the image. Patch is downscaled to the desired image size (96$\times$96) with bi-cubic interpolation ($p$=1).
\item \textit{Flip:} Flip the image horizontally ($p$=0.5).
\item \textit{Color jitter:} Randomly adjust brightness, contrast, saturation and hue. Factors for these aspects are sampled uniformly from $[0.6, 1.4]$, $[0.6, 1.4]$, $[0.8, 1.2]$ and $[-0.1, 0.1]$, respectively ($p$=0.4).
\item \textit{Grayscale:} Convert to grayscale ($p$=0.1).
\item \textit{Gaussian blur:} Gaussian blurring with a blurring radius between 0.1 and 2.
\item \textit{Solarization:} Solarize image by inverting all pixel values above threshold ($p$=0.2).
\end{enumerate}

For the first global crop in the DINO framework, \textit{Random crop global}, \textit{Flip}, \textit{Color jitter} or \textit{Grayscale} and \textit{Gaussian blur} ($p$=1.0) are applied, while for the second global crop, \textit{Gaussian blur} ($p$=0.1) and \textit{Solarization} are applied instead of the \textit{Gaussian blur} with unity probability. For the local crops, \textit{Random crop local}, \textit{Flip}, \textit{Color jitter} or \textit{Grayscale} and \textit{Gaussian blur} ($p$=0.5) are applied. The data augmentation techniques are followed by channel-wise normalization with ImageNet statistics.

\subsubsection{Domain-specific SSL pre-training: DSA set}
The domain-specific set of data augmentation techniques in the DINO SSL framework~\citep{DINO} applied during pre-training consists of:

\begin{enumerate}[noitemsep]
\item \textit{Random crop global:} Randomly take a crop within a [0.4, 1.0] scale of the image. Patch is downscaled to the desired image size (256$\times$256) with bi-cubic interpolation ($p$=1).
\item \textit{Random crop local:} Randomly take a crop within a [0.05, 0.4] scale of the image. Patch is downscaled to the desired image size (96$\times$96) with bi-cubic interpolation ($p$=1).
\item \textit{Flip:} Flip the image horizontally and/or vertically ($p$=0.5).
\item \textit{Motion blur:} Apply motion blurring with a blurring limit randomly sampled from either range of $[9, 9]$, $[11, 11]$, $[17,17]$, $[21, 21]$ and $[25, 25]$.
\item \textit{Zoom blur:} Apply zoom blurring with a maximum factor randomly sampled from either range of $[1.01, 1.02]$, $[1.03, 1.04]$, $[1.05, 1.06]$, $[1.07, 1.08]$ and $[1.09, 1.1]$.
\item \textit{Lens blur:} Apply lens blurring with a blurring limit randomly sampled from either range of $[1, 1]$, $[3, 3]$, $[5, 5]$, $[7, 7]$ and $[9, 9]$.
\item \textit{Median blur:} Apply median blurring with a maximum aperture linear size randomly sampled from either range of $[1, 1]$, $[3, 3]$, $[5, 5]$, $[7, 7]$ and $[9, 9]$.
\item \textit{Increased sharpness:} Increase the sharpness with visibility and lightness of the sharpened image randomly sampled from either range of $[0.1, 0.2]$, $[0.2, 0.3]$, $[0.3, 0.4]$, $[0.4, 0.5]$ and $[0.5, 0.6]$ ($p$=0.1).
\item \textit{Decreased sharpness:} Decrease the sharpness with visibility randomly sampled from either range of $[0.1, 0.2]$, $[0.2, 0.3]$, $[0.3, 0.4]$, $[0.4, 0.5]$ and $[0.5, 0.6]$, and the Gaussian kernel size for blurring randomly sampled from either range of $[3, 3]$, $[5, 5]$, $[7, 7]$, $[9, 9]$ and $[11, 11]$ ($p$=0.1).
\item \textit{Increased contrast:} Increase contrast with factor randomly sampled from either range of $[1.01, 1.1]$, $[1.11, 1.2]$, $[1.21, 1.25]$, $[1.26, 1.3]$ and $[1.31, 1.4]$ ($p$=0.4).
\item \textit{Decreased contrast:} Decrease contrast with factor randomly sampled from either range of $[0.95, 0.99]$, $[0.9, 0.94]$, $[0.85, 0.89]$, $[0.75, 0.84]$ and $[0.65, 0.74]$ ($p$=0.4).
\item \textit{Increased brightness:} Increase brightness with factor randomly sampled from either range of $[1.01, 1.2]$, $[1.21, 1.4]$, $[1.41, 1.6]$, $[1.61, 1.8]$ and $[1.81, 2.0]$ ($p$=0.4).
\item \textit{Decreased brightness:} Decrease brightness with factor randomly sampled from either range of $[0.9, 0.99]$, $[0.85, 0.89]$, $[0.8, 0.84]$, $[0.75, 0.79]$ and $[0.7, 0.74]$ ($p$=0.4).
\item \textit{Increased saturation:} Increase saturation with factor randomly sampled from either range of $[1.01, 1.05]$, $[1.06, 1.1]$, $[1.11, 1.15]$, $[1.16, 1.2]$ and $[1.21, 1.25]$ ($p$=0.4).
\item \textit{Decreased saturation:} Decrease saturation with factor randomly sampled from either range of $[0.9, 0.99]$, $[0.8, 0.89]$, $[0.7, 0.79]$, $[0.6, 0.69]$ and $[0.5, 0.59]$ ($p$=0.4).
\item \textit{Hue red:} Apply jitter in red color spectrum with factor randomly sampled from either range of $[0.0, 0.01]$, $[0.011, 0.013]$, $[0.014, 0.016]$, $[0.017, 0.018]$ and $[0.019, 0.02]$ ($p$=0.4).
\item \textit{Hue green:} Apply jitter in green color spectrum with factor randomly sampled from either range of $[-0.01, 0.0]$, $[-0.013, -0.011]$, $[-0.016, -0.014]$, $[-0.02, -0.017]$ and $[-0.025, -0.021]$ ($p$=0.4).
\end{enumerate}

For the first global crop in the DINO framework, \textit{Random crop global}, \textit{Color jitter}, \textit{Flip}, \textit{Increased} / \textit{Decreased Contrast}, \textit{Increased} / \textit{Decreased Brightness}, \textit{Increased} / \textit{Decreased Saturation}, \textit{Hue red} /  \textit{green} and \textit{Motion} / \textit{Zoom} / \textit{Lens} / \textit{Median blur} ($p$=0.25) are applied. For the second global crop, \textit{Motion} / \textit{Zoom} / \textit{Lens} / \textit{Median blur} ($p$=0.025) and additionally \textit{Increased} / \textit{Decreased Sharpness} compared to the first global crop. For the local crops, \textit{Random crop local}, \textit{Increased} / \textit{Decreased Contrast}, \textit{Increased} / \textit{Decreased Brightness}, \textit{Increased} / \textit{Decreased Saturation}, \textit{Hue red} /  \textit{green} and \textit{Motion} / \textit{Zoom} / \textit{Lens} / \textit{Median blur} ($p$=0.125) are applied. The data augmentation techniques are followed by channel-wise normalization with the normalization values specified in Section~\ref{sec: Supplementary-Preprocess-Normalization}.

\section{Results training with additional video frames}
\label{sec: Supplementary-VideoFrames}
The classification, classification-by-segmentation and localization performance results regarding experiments discussed in Sections~\ref{sec: ExperimentalSetup-Training-VideoFrames} and \ref{sec: ResultsDiscussion-Training-VideoFrames} are displayed in Table~\ref{table: Supplementary-VideoFrames}. 

\begin{table*}
    \centering
        \caption{Classification, classification-by-segmentation and localization performance of the optimal network architecture using previously selected training design choices with considered additional video frame strategies, on the different validation sets. Results are presented as Mean $\pm$ Std. The best results are highlighted in boldface.}
        \begin{tabular}{ l | c c c c c c c}
             \toprule
              \textbf{Additional frames} &\multicolumn{3}{ c }{\textbf{Images + HQ Frames}} & \multicolumn{2}{ c }{\textbf{MQ Frames}} & \multicolumn{2}{ c }{\textbf{LQ Frames}} \\
             \cmidrule{2-4}
             \cmidrule(lr){5-6}
             \cmidrule(lr){7-8}
             & AUROC$_{cls}$ & AUPRC$_{cls}$ & $mD_i$ & AUROC$_{cls}$ & AUPRC$_{cls}$ & AUROC$_{cls}$ & AUPRC$_{cls}$ \\
             \midrule
             No Frames          & \textbf{0.974\sd{.004}} & \textbf{0.973\sd{.003}} & 0.617\sd{.017} & 0.962\sd{.003} & 0.968\sd{.003} & 0.889\sd{.014} & 0.884\sd{.013}\\
             +100\% HQ          & 0.969\sd{.005} & 0.971\sd{.004} & 0.615\sd{.013} & 0.956\sd{.008} & 0.964\sd{.005} & 0.881\sd{.015} & 0.880\sd{.012}\\
             +~~50\% HQ         & 0.971\sd{.003} & 0.972\sd{.003} & 0.623\sd{.011} & 0.960\sd{.004} & 0.967\sd{.003} & 0.889\sd{.012} & 0.886\sd{.013}\\
             +~~10\% HQ         & 0.968\sd{.006} & 0.970\sd{.006} & 0.623\sd{.013} & 0.956\sd{.007} & 0.965\sd{.006} & 0.877\sd{.020} & 0.879\sd{.017}\\
             +100\% MQ          & 0.970\sd{.008} & 0.972\sd{.007} & 0.628\sd{.009} & 0.954\sd{.009} & 0.963\sd{.008} & 0.879\sd{.017} & 0.880\sd{.016}\\
             +~~50\% MQ         & 0.971\sd{.005} & 0.970\sd{.006} & 0.625\sd{.007} & 0.960\sd{.008} & 0.967\sd{.005} & 0.881\sd{.015} & 0.881\sd{.015}\\
             +~~10\% MQ         & 0.971\sd{.006} & 0.971\sd{.006} & 0.621\sd{.019} & 0.959\sd{.006} & 0.966\sd{.005} & 0.887\sd{.016} & 0.884\sd{.018}\\
             +100\% LQ          & 0.962\sd{.013} & 0.963\sd{.013} & 0.607\sd{.073} & 0.951\sd{.015} & 0.960\sd{.013} & 0.877\sd{.024} & 0.874\sd{.026}\\
             +~~50\% LQ         & 0.972\sd{.004} & 0.971\sd{.004} & 0.632\sd{.016} & 0.960\sd{.002} & 0.966\sd{.002} & 0.881\sd{.011} & 0.874\sd{.012}\\
             +~~10\% LQ         & 0.964\sd{.011} & 0.965\sd{.009} & 0.588\sd{.076} & 0.950\sd{.009} & 0.960\sd{.010} & 0.851\sd{.011} & 0.850\sd{.016}\\
             +100\% HQ - MQ    & 0.965\sd{.004} & 0.969\sd{.003} & 0.606\sd{.022} & 0.950\sd{.010} & 0.960\sd{.007} & 0.863\sd{.033} & 0.869\sd{.025}\\
             +~~50\% HQ - MQ   & 0.969\sd{.005} & 0.971\sd{.005} & 0.632\sd{.012} & 0.956\sd{.008} & 0.964\sd{.007} & 0.878\sd{.027} & 0.879\sd{.021}\\
             +~~10\% HQ - MQ   & 0.971\sd{.005} & 0.971\sd{.004} & 0.619\sd{.009} & \textbf{0.963\sd{.002}} & \textbf{0.969\sd{.001}} & \textbf{0.893\sd{.010}} & \textbf{0.888\sd{.011}}\\
             +100\% HQ - LQ    & 0.964\sd{.017} & 0.967\sd{.016} & 0.591\sd{.059} & 0.954\sd{.009} & 0.963\sd{.010} & 0.874\sd{.018} & 0.873\sd{.019}\\
             +~~50\% HQ - LQ   & 0.959\sd{.019} & 0.961\sd{.016} & 0.570\sd{.087} & 0.949\sd{.012} & 0.958\sd{.010} & 0.869\sd{.025} & 0.865\sd{.025}\\
             +~~10\% HQ - LQ   & 0.967\sd{.009} & 0.968\sd{.009} & 0.602\sd{.092} & 0.955\sd{.010} & 0.963\sd{.010} & 0.863\sd{.024} & 0.860\sd{.020}\\
             +100\% MQ - LQ    & 0.951\sd{.016} & 0.953\sd{.018} & 0.589\sd{.050} & 0.936\sd{.014} & 0.949\sd{.014} & 0.852\sd{.031} & 0.855\sd{.027}\\
             +~~50\% MQ - LQ   & 0.963\sd{.011} & 0.966\sd{.009} & 0.577\sd{.065} & 0.959\sd{.009} & 0.961\sd{.008} & 0.870\sd{.020} & 0.866\sd{.018}\\
             +~~10\% MQ - LQ   & 0.973\sd{.002} & 0.972\sd{.002} & \textbf{0.640\sd{.013}} & 0.959\sd{.004} & 0.966\sd{.003} & 0.873\sd{.017} & 0.869\sd{.017}\\
            \midrule
            \midrule
             \textbf{Additional frames} & \multicolumn{3}{ c }{\textbf{Images + HQ Frames}} & \multicolumn{2}{ c }{\textbf{MQ Frames}} & \multicolumn{2}{ c }{\textbf{LQ Frames}} \\
             \cmidrule{2-4}
             \cmidrule(lr){5-6}
             \cmidrule(lr){7-8}
             & AUROC$_{seg}$ & AUPRC$_{seg}$ & & AUROC$_{seg}$ & AUPRC$_{seg}$ & AUROC$_{seg}$ & AUPRC$_{seg}$ \\
             \midrule
             No Frames          & 0.975\sd{.003} & 0.974\sd{.004} & & 0.961\sd{.004} & 0.964\sd{.004} & 0.879\sd{.011} & 0.871\sd{.011} \\
             +100\% HQ          & 0.972\sd{.004} & 0.973\sd{.004} &  & 0.958\sd{.007} & 0.964\sd{.004} & 0.874\sd{.017} & 0.871\sd{.015}\\
             +~~50\% HQ         & 0.974\sd{.001} & 0.973\sd{.001} &  & 0.964\sd{.005} & 0.967\sd{.003} & 0.883\sd{.020} & 0.878\sd{.016}\\
             +~~10\% HQ         & 0.972\sd{.006} & 0.973\sd{.006} &  & 0.961\sd{.003} & 0.965\sd{.005} & 0.878\sd{.024} & 0.875\sd{.021}\\
             +100\% MQ          & 0.974\sd{.005} & \textbf{0.975\sd{.004}} &  & 0.959\sd{.007} & 0.964\sd{.004} & 0.883\sd{.010} & 0.886\sd{.010}\\
             +~~50\% MQ         & 0.974\sd{.004} & 0.974\sd{.004} &  & 0.962\sd{.006} & 0.966\sd{.003} & 0.884\sd{.018} & 0.881\sd{.014}\\
             +~~10\% MQ         & 0.973\sd{.007} & 0.971\sd{.007} &  & 0.961\sd{.006} & 0.964\sd{.006} & 0.888\sd{.019} & 0.880\sd{.023}\\
             +100\% LQ          & 0.965\sd{.012} & 0.966\sd{.010} &  & 0.954\sd{.016} & 0.960\sd{.013} & 0.892\sd{.047} & 0.887\sd{.044}\\
             +~~50\% LQ         & 0.972\sd{.004} & 0.971\sd{.004} &  & 0.962\sd{.004} & 0.964\sd{.002} & \textbf{0.899\sd{.011}} & \textbf{0.890\sd{.009}}\\
             +~~10\% LQ         & 0.968\sd{.006} & 0.967\sd{.007} &  & 0.957\sd{.006} & 0.961\sd{.008} & 0.873\sd{.019} & 0.867\sd{.022}\\
             +100\% HQ - MQ    & 0.972\sd{.004} & 0.973\sd{.003} &  & 0.956\sd{.005} & 0.964\sd{.004} & 0.880\sd{.022} & 0.879\sd{.019}\\
             +~~50\% HQ - MQ   & 0.975\sd{.005} & \textbf{0.975\sd{.005}} &  & 0.962\sd{.006} & 0.967\sd{.006} & 0.884\sd{.026} & 0.883\sd{.020}\\
             +~~10\% HQ - MQ   & 0.974\sd{.002} & 0.973\sd{.003} &  & \textbf{0.966\sd{.003}} & \textbf{0.968\sd{.002}} & 0.890\sd{.015} & 0.882\sd{.012}\\
             +100\% HQ - LQ    & 0.970\sd{.011} & 0.971\sd{.012} &  & 0.959\sd{.007} & 0.964\sd{.009} & 0.896\sd{.021} & 0.889\sd{.027}\\
             +~~50\% HQ - LQ   & 0.966\sd{.011} & 0.966\sd{.012} &  & 0.955\sd{.007} & 0.960\sd{.008} & 0.889\sd{.028} & 0.875\sd{.032}\\
             +~~10\% HQ - LQ   & 0.969\sd{.006} & 0.968\sd{.008} &  & 0.959\sd{.008} & 0.962\sd{.009} & 0.880\sd{.025} & 0.868\sd{.026}\\
             +100\% MQ - LQ    & 0.963\sd{.010} & 0.964\sd{.009} &  & 0.951\sd{.012} & 0.957\sd{.011} & 0.871\sd{.028} & 0.868\sd{.027}\\
             +~~50\% MQ - LQ   & 0.968\sd{.008} & 0.968\sd{.008} &  & 0.957\sd{.005} & 0.962\sd{.004} & 0.889\sd{.021} & 0.881\sd{.021}\\
             +~~10\% MQ - LQ   & \textbf{0.976\sd{.002}} & 0.974\sd{.003} &  & 0.964\sd{.004} & 0.965\sd{.004} & 0.891\sd{.029} & 0.882\sd{.025}\\
             \bottomrule
        \end{tabular}
    \label{table: Supplementary-VideoFrames}
\end{table*}
